# Supplementary material for: Language Models are Causal Knowledge Extractors for Zero-shot Video Question Answering
Source: arXiv:2304.03754 source file (2023-04-07)
Supplement: Supplementary file 1 [file A-appendix.tex]

\section{Video QA Settings}
%\paragraph{Video QA training}
In all experiments, we follow NExT-QA \cite{dataset_xiao2021nextqa} to preprocess videos where 8 segments with 16 consecutive frames are uniformly sampled. For visual features, ImageNet \cite{deng2009imagenet} pre-trained Resnet101 \cite{resnet_he2016residual} and Kinetics \cite{kay2017kinetics} pre-trained inflated 3D ResNeXt-101 \cite{3dresnet_hara3dcnns} are used as feature extractors. To extract question and answer features, we follow the setting of NExT-QA and further pre-train the BERT \cite{devlin-etal-2019-bert} on our generated training set and extract QA features. To adapt an open-ended QA model for multi-choice QA, we follow the NExT-QA implementation and concatenate each candidate answer with the question, and optimize it with Hinge Loss.

 For video QA training, we employ the default NeXT-QA implementation\footnote{https://github.com/doc-doc/NExT-QA
 %, 6b5a380 committed on Aug 6, 2022
 } with the exception of setting the \textit{patience} in the \textit{ReduceLROnPlateau} to 2 instead of 5, and the maximum number of epochs to 25 instead of 50, as we observed a faster convergence during training. We conduct the training on a single NVIDIA TITAN RTX GPU, and each experiment takes around 18 to 24 hours.
%For hyper-parameters, we use the default ones of NeXT-QA\footnote{https://github.com/doc-doc/NExT-QA} implementation except that we set \textit{patience} in \textit{ReduceLROnPlateau} to 2 instead of 5 and max epoch to 25 instead of 50 as we observe quick convergence during training. For both models, we train on NVIDIA TITAN RTX GPU, 
%conduct each experiment in a single run, 
%and an experiment takes about 18 to 24 hours.

\begin{figure*}[!ht]
\centering
\includegraphics[width=\linewidth]{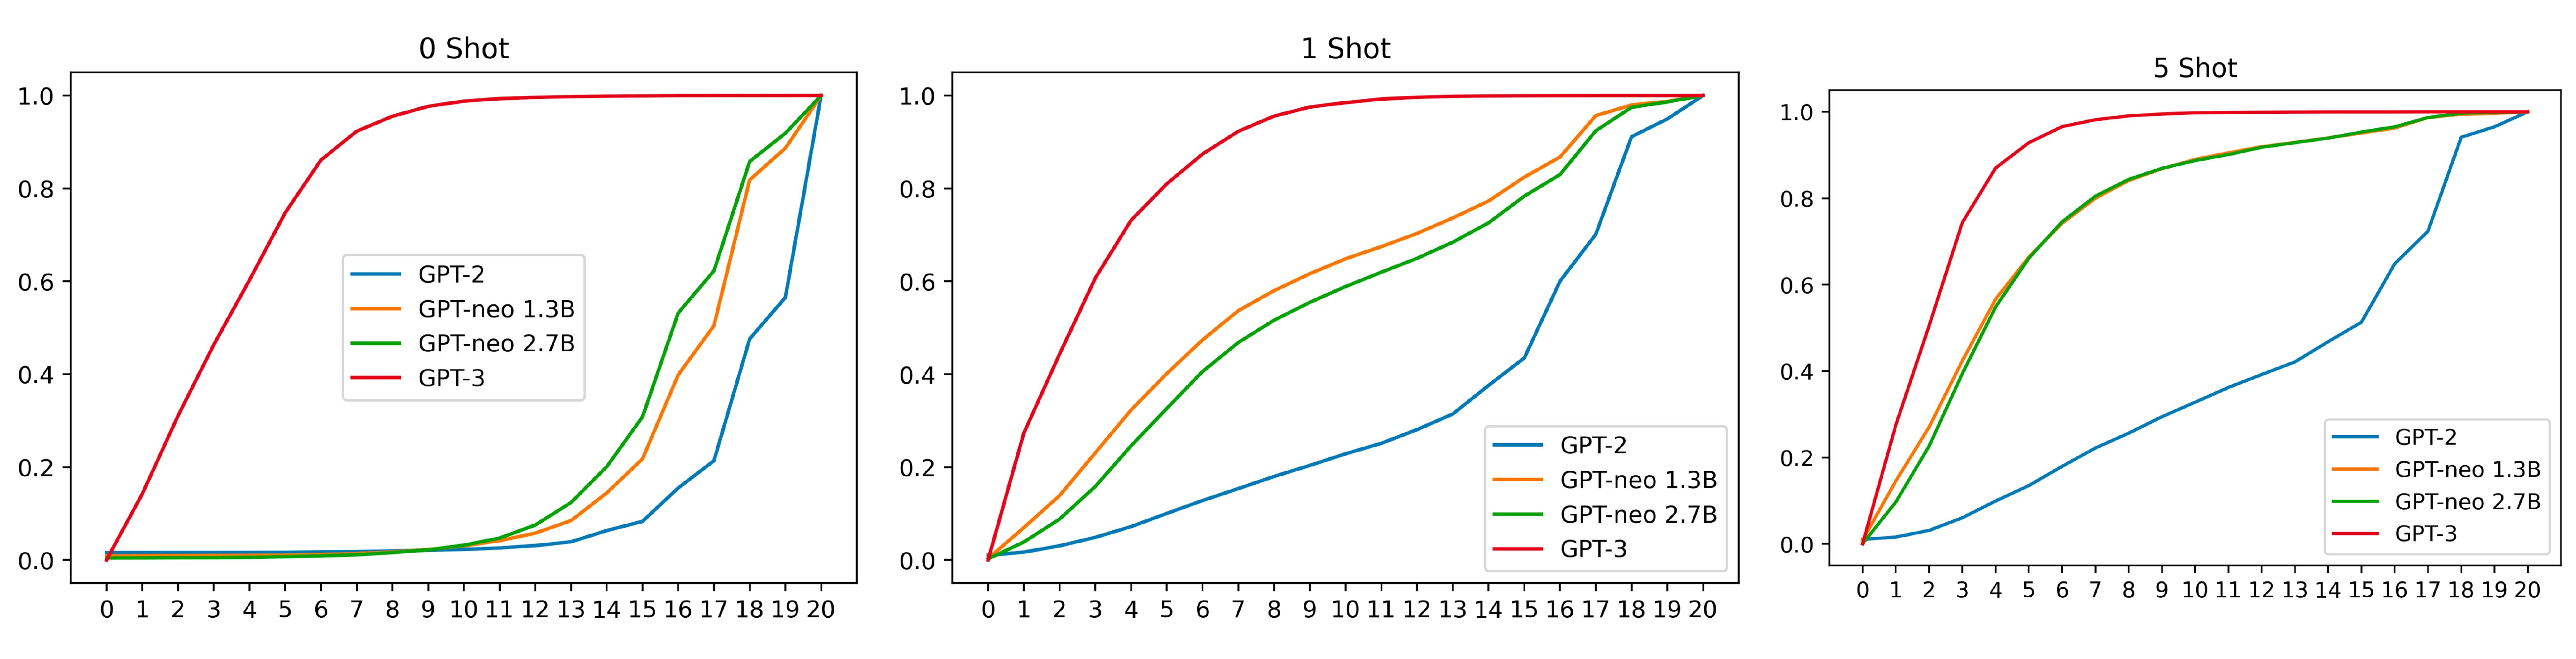}
\caption{\textbf{Cumulative distribution of LM response lengths that reflects LM response quality.} X axis represents the token length of response and Y axis shows the ratio of the dataset. (Section \ref{subsec:LM_ana}) }
\label{lm_dist}
\end{figure*}

\section{LM Output Lengths Distributions as quality indicators} None GPT-3 LMs tends to generate noisy and redundant answers, and few-shot prompting could alleviate this. Figure \ref{lm_dist} displays the cumulative distribution of LM answer lengths. While longer answer might provide more comprehensive detail in theory, we observed that longer answers are usually noisy or redundant, such as providing irrelevant details, copying, paraphrasing, or even completely neglect the prompts. Therefore, we use the length distribution\footnote{We use NLTK word tokenizer to tokenize.} of LM answers as an indicator of overall quality. We observe that despite being more noisy and redundant, GPT-Neos are still comparable to GPT-3 as shown in Table \ref{tab:prompt_result}. We hypothesis that multi-choice QA model could still capture key information from noisy input and enables the training. Also, noisy answers does not follow answer patterns in \taskabbr{} so the model will not be biased. However, for generation tasks such as video captioning, GPT-3 might be a supreme solution.
